# Supplementary material for: Dissolution of topological Fermi arcs in a dirty Weyl semimetal
Source: arXiv:1703.09706 ancillary file (2017-11-08)
Supplement: Supplementary file 1 [file arxiv-SOM-FermiArcs-final.pdf]

# Supplementary Materials for "Dissolution of topological Fermi arcs in a dirty Weyl semimetal"

Robert-Jan Slager,[1] Vladimir Juričić,[2] and Bitan Roy[3,4]

[1] *Max-Planck-Institut für Physik komplexer Systeme, Nöthnitzer Str. 38, 01187 Dresden, Germany*
[2] *Nordita, KTH Royal Institute of Technology and Stockholm University, Roslagstullsbacken 23, 10691 Stockholm, Sweden*
[3] *Department of Physics and Astronomy, Rice University, Houston, Texas 77005, USA*
[4] *Condensed Matter Theory Center and Joint Quantum Institute, Department of Physics, University of Maryland, College Park, Maryland 20742- 4111 USA*

**This pdf file includes:**

Supplementary text

Figures S1-S9

References

Supplementary text contains:

**S1.** Details of the algorithm for finding Fermi arc states in clean and disordered Weyl semimetal (WSM);

**S2.** Characterization of the WSM-metal quantum phase transition (QPT) in the bulk of the system;

**S3.** Fermi arc states for the system with linear dimension $L = 100$ and $L = 200$ in the direction of open boundary.

## S1. DETAILS OF THE ALGORITHM FOR CONSTRUCTING TOPOLOGICAL FERMI ARC STATES

We here present the details of the algorithm and numerical methods used to extract the arc states across the Weyl semimetal (WSM)-metal transition. Our numerical analysis is based on the lattice tight-binding model [Eq. (1) in the main text] for a WSM given by

$$H_W(\mathbf{k}) = t\ [\sigma_1 \sin(k_x a) + \sigma_2 \sin(k_y a) + \sigma_3 \cos(k_z a)] + t\ \sigma_3 \big[2 - \cos(k_x a) - \cos(k_y a)\big]. \tag{S1}$$

Here, $\sigma$s are the standard Pauli matrices and the two-component spinor can be chosen as $\Psi_{\mathbf{k}}^{\top} = (\psi_{\mathbf{k},\uparrow}, \psi_{\mathbf{k},\downarrow})$, where $\psi_{\mathbf{k},\uparrow/\downarrow}$ is fermion annihilation operator with momentum $\mathbf{k}$ and spin/pseudo-spin projection $\uparrow$ / $\downarrow$. For numerical analysis we will set $t = 1$, and energy ($E$) and strength of disorder ($W$) is measured in units of $t$.

We consider a cubic lattice with periodic boundary conditions in the $\hat{y}, \hat{z}$ directions, while the translational symmetry is broken in the $\hat{x}$ direction, along which we impose an open boundary. Such a setup allows us to track the Fermi arc surface state on the $(k_y, k_z)$ plane (referred as top and bottom surfaces, and specifically we focus only on the top surface). In the clean system, the spectrum and corresponding wavefunctions in terms of the real space coordinate $x$ and momentum $\mathbf{k}_\perp \equiv (k_y, k_z)$, can directly be calculated using exact diagonalization techniques from the lattice Hamiltonian. The form of this Hamiltonian that we numerically implement reads as

$$\begin{aligned} H = \sum_{j,k_y,k_z} & -\frac{it}{2}\left[\psi^\dagger_{j+1,k_y,k_z,\uparrow}\psi_{j,k_y,k_z,\downarrow} - \psi^\dagger_{j-1,k_y,k_z,\uparrow}\psi_{j,k_y,k_z,\downarrow}\right] - \frac{t}{2}\left[e^{ik_y a}\psi^\dagger_{j,k_y,k_z,\uparrow}\psi_{j,k_y,k_z,\downarrow} - e^{-ik_y a}\psi^\dagger_{j,k_y,k_z,\uparrow}\psi_{j,k_y,k_z,\downarrow}\right] \\ & - \frac{t}{2}\left[\psi^\dagger_{j+1,k_y,k_z,\uparrow}\psi_{j,k_y,k_z,\uparrow} - \psi^\dagger_{j-1,k_y,k_z,\downarrow}\psi_{j,k_y,k_z,\downarrow}\right] - \frac{t}{2}\left[e^{ik_y a}\psi^\dagger_{j,k_y,k_z,\uparrow}\psi_{j,k_y,k_z,\uparrow} - e^{-ik_y a}\psi^\dagger_{j,k_y,k_z,\downarrow}\psi_{j,k_y,k_z,\downarrow}\right] \\ & + \frac{t}{2}\left[e^{ik_z a}\psi^\dagger_{j,k_y,k_z,\uparrow}\psi_{j,k_y,k_z,\uparrow} - e^{ik_z a}\psi^\dagger_{j,k_y,k_z,\downarrow}\psi_{j,k_y,k_z,\downarrow}\right] + t\ \psi^\dagger_{j,k_y,k_z,\uparrow}\psi_{j,k_y,k_z,\uparrow} + t\ \psi^\dagger_{j,k_y,k_z,\downarrow}\psi_{j,k_y,k_z,\downarrow} + H.c. \end{aligned} \tag{S2}$$

where $j$ is the site index in real space in the $\hat{x}$ direction. This Hamiltonian features a block diagonal form in terms of $2L \times 2L$ blocks, where $L$ represents the system size in the $\hat{x}$ direction, and each block depends on the momentum $\mathbf{k}_\perp$ in the periodic directions. The spectrum of this Hamiltonian for the parameters we use in our simulations is shown in Fig. S1A. The resulting Fermi arc for $L = 300$ has been shown in Fig. 2A and Fig. 3A in the main text, while we also display it for $L = 100$ [ Fig. S2A and Fig. S4A] and $L = 200$ [Fig. S3A and Fig. S5A] in this Supplementary Materials. We now discuss the implementation of random change impurities in the momentum space and its correspondence with real space realization.

In the following, we assume that translational symmetry is preserved on average, and the effect of potential disorder or random charge impurities in a WSM is captured by adding the following Hamiltonian to Eq. (S2)

$$H_{\text{dis}} = \sum_{x,k_y,k_z,\sigma} V(x,k_y,k_z)\ \psi^\dagger_{x,k_y,k_z,\sigma}\ \psi_{x,k_y,k_z,\sigma}. \tag{S3}$$

The system size in the momentum space along each periodic direction ($k_y$ and $k_z$) in our calculations is $m_y = m_z = 60$ throughout and the linear dimension of the system along $\hat{x}$ will be denoted by $L$. The random variable $V(x, k_y, k_z)$ is distributed uniformly, randomly and independently within a box distribution in the interval $[-W, W]$ on each site in the $x$-direction in the real space, as well as in the $k_y$ and $k_z$ direction in the momentum space.

Notice that when the disorder potential is evenly distributed within the range $[-W, W]$ in the momentum space in the $(k_y, k_z)$ plane, the corresponding disorder realization in the $(y, z)$ plane, for a given value of $x$, in the real space is

$$|V(\mathbf{r}_\perp - \mathbf{r}'_\perp)|^2 = \frac{1}{W}\int_{-W}^{W} dw \left| \int d^2\mathbf{k}_\perp\ e^{(\mathbf{r}_\perp - \mathbf{r}'_\perp)\cdot\mathbf{k}_\perp}\ w\ \delta\left(\mathbf{k}_\perp\right)\right|^2 = \frac{W^2}{3}, \tag{S4}$$

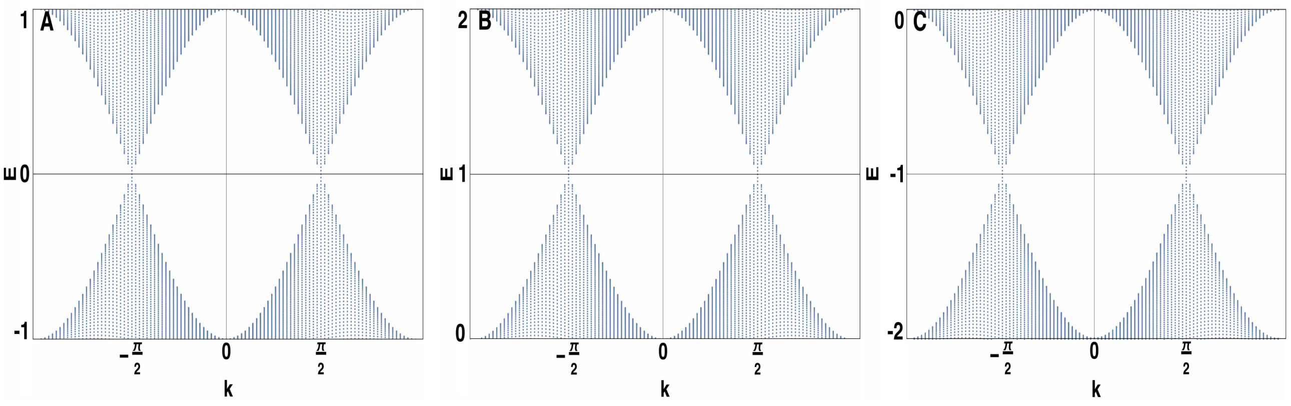

FIG. S1: **(A)** Spectrum of the tight-binding Hamiltonian for Weyl semimetal [Eq. (S1)] obtained by diagonalizing its momentum space representation [Eq. (S2)]. It shows existence of two Weyl points at $\mathbf{k} = \left(0, 0, \frac{\pi}{2a}\right)$ with $a = 1$, around which the dispersion scales linearly with momentum. The Weyl points are located at energy $E = 0$. The same plot, but in the presence of **(B)** a net positive or electron doping $[V(x, k_y, k_z) = +1]$ and **(C)** a net negative or hole doping $[V(x, k_y, k_z) = -1]$ from the construction discussed in Sec. S1 [see also Eq. (S3)]. Panels **(B)** and **(C)** show that in the momentum-space representation of the tight-binding model for Weyl semimetal the presence of a constant chemical potential causes only an overall shift of the energy.

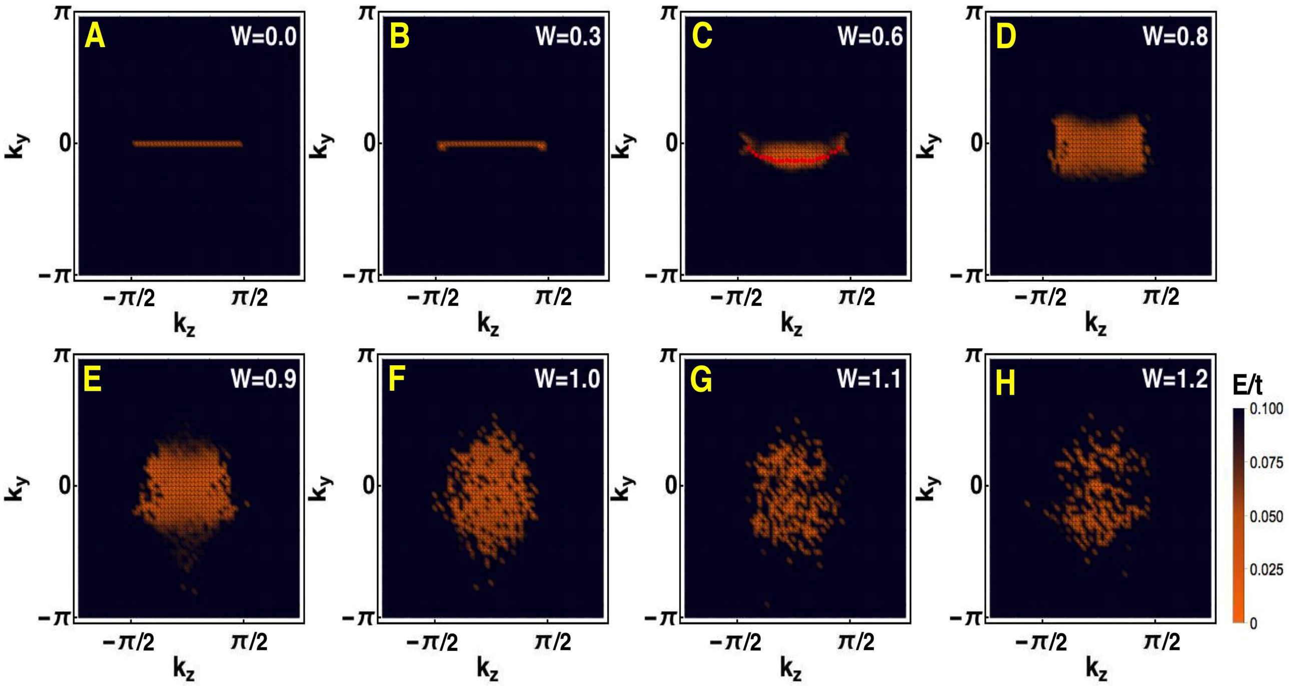

FIG. S2: Evolution of one dimensional chiral edge states on the top surface residing between two Weyl points, located at $\pm\frac{\pi}{2a}$ (with $a = 1$) in the clean system, with increasing strength of disorder $W$ (quoted in each panel), within the energy window $|E| \leq 0.1\, t$ for the system size $L = 100$ in the open direction. The red dotted line in **(C)** for $W = 0.6$ marks the Fermi arc.

and, hence constant, where $\mathbf{r}_\perp \equiv (y, z)$. Therefore, the disorder distribution we implement to demonstrate the evolution of the Fermi arc with gradual onset of the randomness in the system, assumes a *stacked planar* construction in real space. More specifically, for each discrete value of $\hat{x}$ coordinate there is no variation of the onsite potential in the $(y, z)$ plane, while the disorder distribution is completely random in the $\hat{x}$ direction. Such a stacked planar construction allows us to access exact eigenstates and eigenenergies in sufficiently large systems that may not be accessible otherwise. In the next section we will provide explicit numerical evidence that such

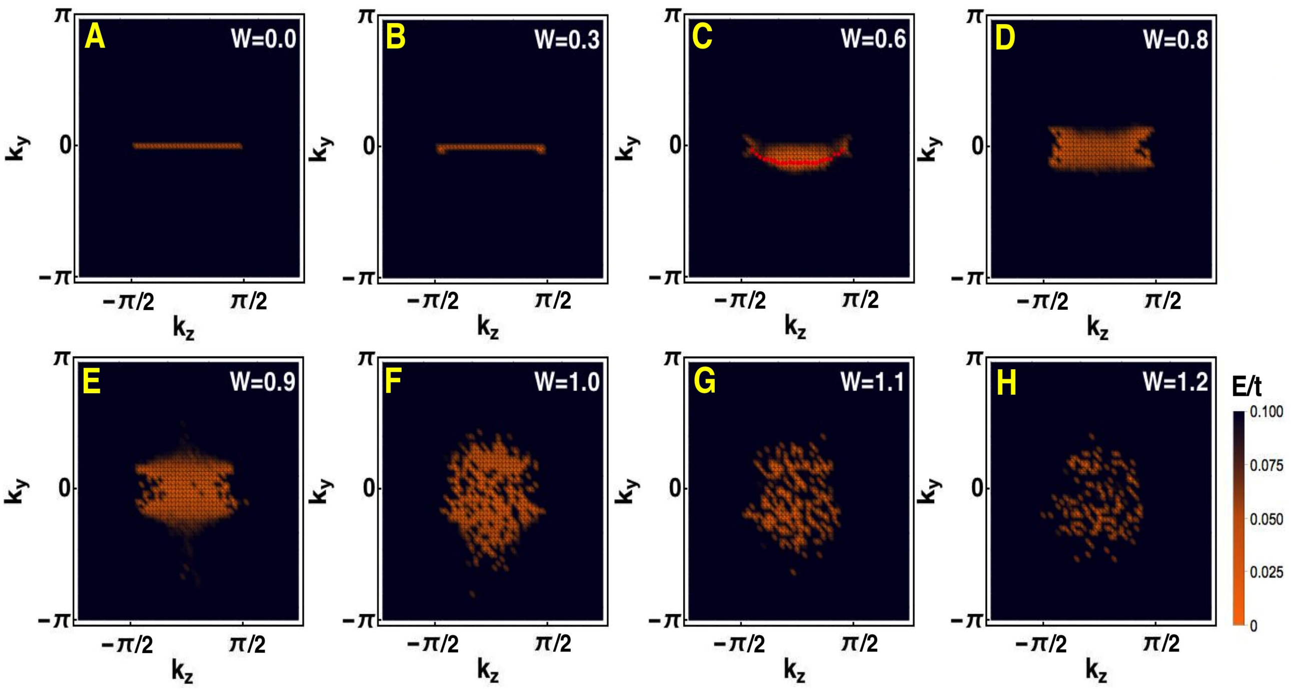


FIG. S3: Evolution of one dimensional chiral edge states on the top surface residing between two Weyl points, located at $\pm\frac{\pi}{2a}$ (with $a = 1$) in the clean system, with increasing strength of disorder $W$ (quoted in each panel), within the energy window $|E| \leq 0.1\ t$ for the system size $L = 200$ in the open direction. The red dotted line in **(C)** for $W = 0.6$ marks the Fermi arc.

*stacked planar* construction does not change the universality class of the WSM-metal quantum phase transition (QPT).

To check the implementation of the chemical potential disorder explicitly, we first show the plot of the energy spectrum of the Hamiltonian [Eq. S2] with a constant $V(x, k_y, k_z) = V$ in Eq. (S3), taking values $V = \pm 1$ (in units of hopping parameter $t$), which expectedly produces only a global shift in energy, as shown in Figs. S1B and S1C, respectively. Next we describe the algorithm to extract surface states in a disordered WSM when $V(x, k_y, k_z)$ is a random variable at each site of the real and momentum space and distributed uniformly and randomly within the range $[-W, W]$.

Upon introducing random charge impurities with the distribution highlighted above, we subsequently sort the eigenstates according to energy and perform an average over 600 disorder realizations to obtain a spectrum of average energies and corresponding normalized wavefunctions. In this averaging procedure we keep track of the relative overlap of the wavefunctions and ensure that orthogonal states close in energy are not averaged over.

We extract the arc states of a system with open boundary conditions in the $\hat{x}$ direction. For concreteness we only consider the top surface and select the state with a momentum $\mathbf{k}_\perp = (k_y, k_z)$ that displays the largest weight $A(\mathbf{k}_\perp)$ given by

$$A_t(\mathbf{k}_\perp) = \sqrt{\psi_\uparrow(x_t, \mathbf{k}_\perp)^* \, \psi_\uparrow(x_t, \mathbf{k}_\perp) + \psi_\downarrow(x_t, \mathbf{k}_\perp)^* \, \psi_\downarrow(x_t, \mathbf{k}_\perp)}, \tag{S5}$$

where the top surface is at $x = x_t$ and the spin/pseudo-spin indices ($\uparrow$ and $\downarrow$) are explicitly labeled. Considering the clean system first, we find a band of highly localized states with $A_t \sim 1$, as a function of the momentum $\mathbf{k}_\perp$. We then find the Fermi arc as a zero-energy sub-band in this set of localized surface states, which connects the projected Weyl points $(k_y, k_z) = (0, \pm\frac{\pi}{2a})$ on the surface Brillouin zone (SBZ), see Figs. 2A and 3A in the main text, and Figs. S2A, S3A, S4A, S5A in this Supplementary Materials.

We apply the same procedure in the presence of disorder by using the fact that the momentum $\mathbf{k}_\perp = (k_y, k_z)$ can be considered as a good quantum number, but only on average. We select the highest localized states for each momentum in the SBZ and then take a small energy window $|\Delta E| = 0.1\ t$ around zero energy, such that we obtain a connected patch of one-dimensional chiral edge states; the locus of the zero energy modes constitutes the topological

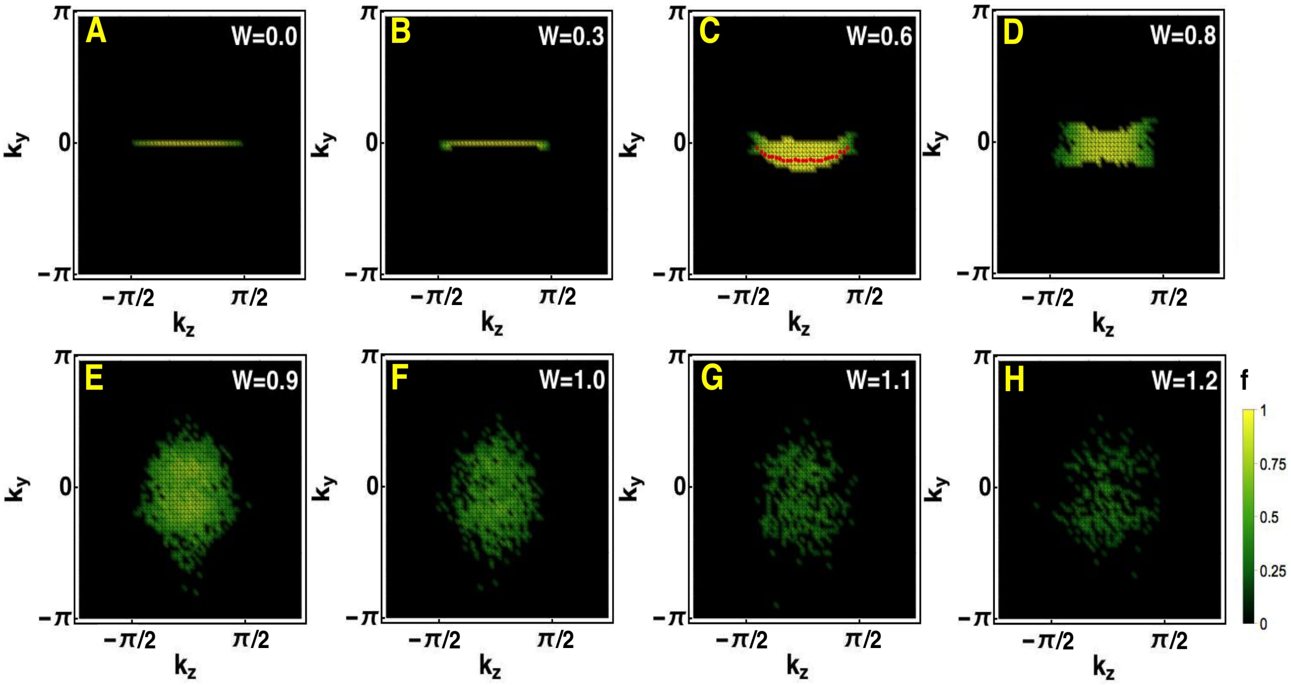


FIG. S4: Fraction of the wave-function ($f$) localized on the top surface for the same set of low-energy states and strength of disorder as in Fig. S2 in a system with linear dimension $L = 100$ along the direction of open boundary. The red dotted line in **(C)** for $W = 0.6$ marks the Fermi arc.

Fermi arcs. As long as it is possible to obtain such a connected patch of one dimensional chiral edge states localized on the SBZ we can construct the Fermi arc. The results have already been displayed in Fig. 2 and Fig. 3 of the main text for $L = 300$. In this Supplementary Materials we also display analogous figures for systems with $L = 100$ [ Figs. S2 and S4] and $L = 200$ [Figs. S3 and S5]. We will return to the discussion on the evolution of the Fermi arc in Sec. S3. We next discuss the WSM-metal QPT in the bulk of a WSM that together with the dissolution of Fermi arc promotes the bulk-boundary correspondence across this transition.

## S2. WEYL SEMIMETAL-METAL QUANTUM PHASE TRANSITION IN THE BULK

To corroborate our analysis on gradual dissolution of the Fermi arcs as the system approaches the WSM-metal quantum critical point (QCP), we also consider the disorder driven WSM-metal QPT in the bulk of the system by imposing the periodic boundary conditions in all three directions. Understanding the role of disorder in WSM (and other closely related systems that also support linearly dispersing quasiparticles such as Dirac semimetal) and the possibility of a strong disorder driven WSM-metal QPT has culminated in a surge of analytical [1–16] and numerical [17–31] works in recent past. We here focus on the scaling of average density of states (ADOS) in the bulk of a WSM with gradual increment of randomness in the system, which serves as a bonafide order-parameter (OP) across the transition. We perform this analysis in two different setups: (i) By directly computing the ADOS from $H + H_{dis}$ in a mixed real and momentum space representation, highlighted in the previous section, (ii) by computing the ADOS using well established kernel polynomial method (KPM) in real space with stacked planar construction of disorder realization [32] [see Eq. (S4) and discussion therein]. The scaling of ADOS obtained from these two methods is respectively shown in Fig. S6A and Figs. S6B and S6C. Now we proceed with the analysis of ADOS and establish that both methods reveal the same universality class of the WSM-metal QPT. Most importantly, we also demonstrate that the location of the WSM-metal QPT are identical in these two methods.

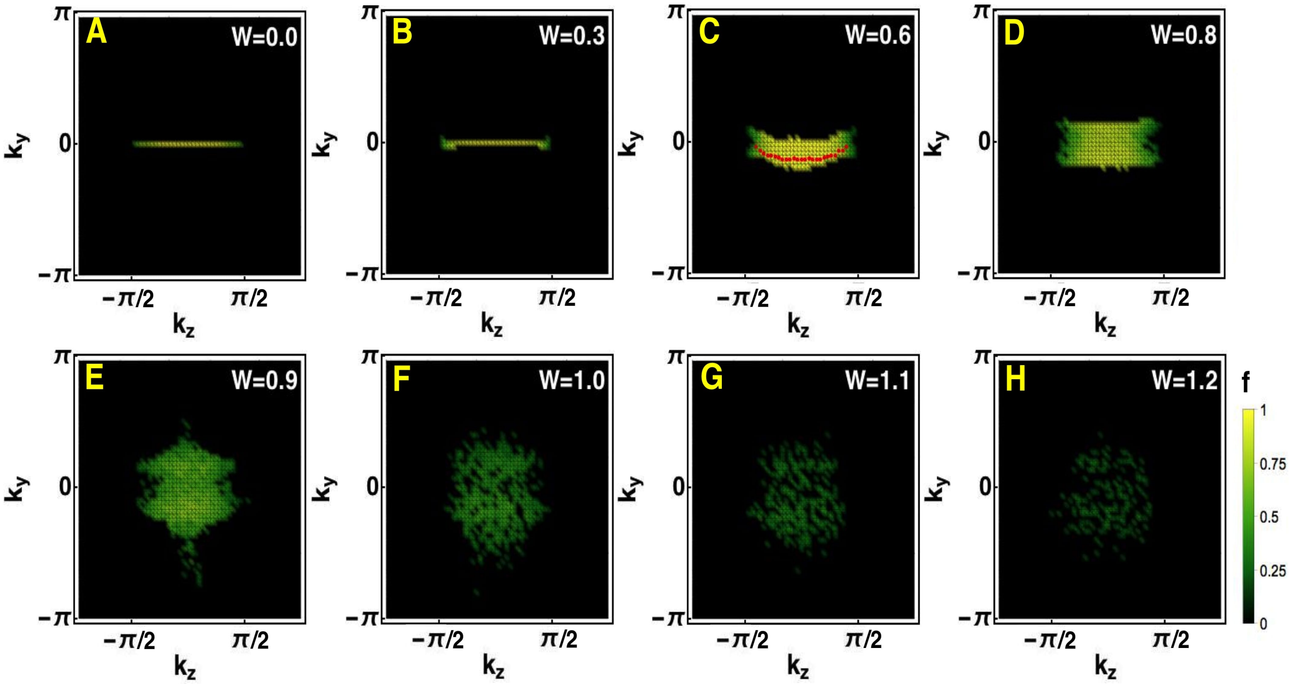


FIG. S5: Fraction of the wave-function ($f$) localized on the top surface for the same set of low-energy states and strength of disorder as in Fig. S3 in a system with linear dimension $L = 200$ along the direction of open boundary. The red dotted line in **(C)** for $W = 0.6$ marks the Fermi arc.

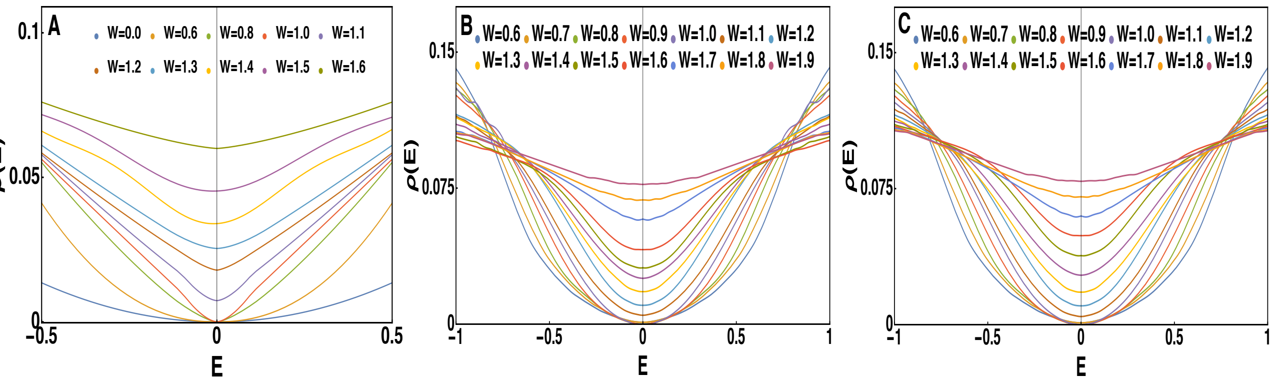


FIG. S6: The scaling of average density of states with varying strength of potential disorder ($W$) obtained from **(A)** diagonalization of $H + H_{dis}$ [see Eq. (S2) and Eq. (S3), and Sec S1 for discussion]. Dimensionality of real and momentum space lattice for numerical analysis is $L = 300, m_y = m_z = 60$. Panels **(B)** and **(C)** display the same quantity obtained by employing kernel polynomial method in real space with stacked planar construction of disorder along $\hat{x}$ and $\hat{z}$ direction [highlighted as (i) and (ii) in Sec. S2 B], respectively. The system size is $L_x \times L_y \times L_z = 3000 \times 30 \times 30$ and $L_x \times L_y \times L_z = 30 \times 30 \times 3000$, respectively, for **(B)** and **(C)**.

### A. Direct computation of ADOS

We first compute the ADOS following the methodology (i) highlighted above, and locate the WSM-metal critical point ($W_c$), extract the values of the dynamical critical exponent (DSE) ($z$) and the correlation length exponent (CLE) ($\nu$) using the scaling analysis of ADOS, which we present below. The central results of our analysis from the form of ADOS shown in Fig. S6A are summarized in Fig. S7. We perform disorder averaging over 600 independent disorder realizations.

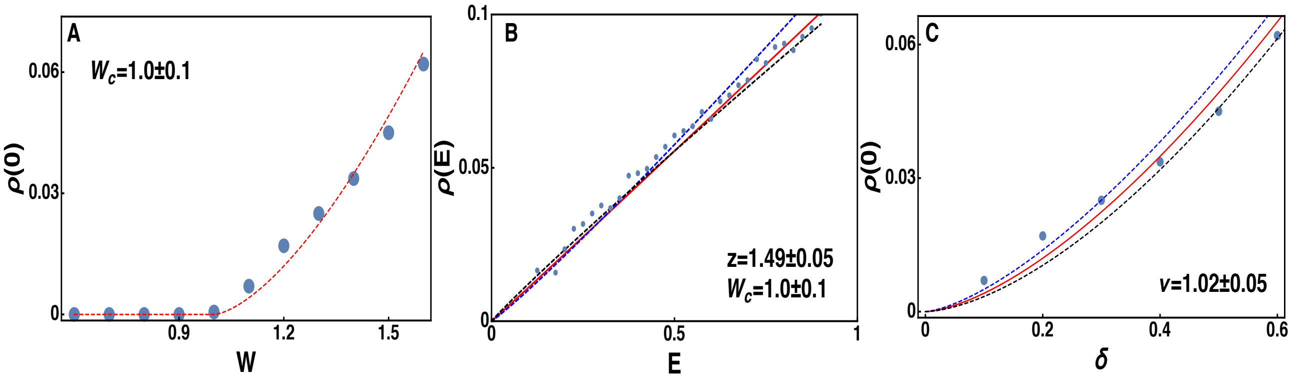


FIG. S7: **(A)** Scaling of average density of states (ADOS) at zero energy [$\varrho(0)$] vs. disorder ($W$) in the bulk of a Weyl semimetal, giving the critical strength of disorder ($W_c$) for Weyl semimetal-metal quantum phase transition $W_c = 1 \pm 0.1$. **(B)** Scaling of ADOS with energy $E$ for $W = W_c$, yielding the dynamic scaling exponent at this transition $z = 1.49 \pm 0.05$. **(C)** Scaling of ADOS at zero energy [$\varrho(0)$] vs. $\delta \left(= \frac{W-W_c}{W_c}\right)$, yielding the correlation length exponent $\nu = 1.02 \pm 0.05$. We here impose periodic boundary conditions in all three directions [see Sec. S2 A for a discussion].

The general scaling theory mandates the following scaling form of the ADOS in a disordered WSM as a function of energy $E$, the linear dimensionality of the system $L$ and the reduced distance from the QCP $\delta = \frac{W-W_c}{W_c}$

$$\varrho(E, L) = \delta^{\nu(d-z)} \, F\left(|E|\delta^{-\nu z}, \delta L^{1/\nu}\right), \tag{S6}$$

where $F$ is a universal, but typically unknown scaling function. [1, 3, 5, 6, 8, 17, 19, 21, 22, 24] We here analyze the behavior of the scaling function in semimetallic, quantum critical and metallic regimes of the phase diagram of a dirty WSM for sufficiently large systems, so that we can neglect the finite size corrections to the scaling function $F$ and work in the limit $L \to \infty$. As demonstrated below, the scaling of ADOS allows us to extract critical exponents $z$ and $\nu$ at the WSM-metal QCP.

First, we focus on the ADOS at zero energy [$\varrho(0)$], as a function of disorder ($W$), as shown in Fig. S7A. Notice that $\varrho(0)$ is pinned to zero for weak enough disorder while beyond a critical strength of disorder, which we find to be $W_c = 1.0 \pm 0.1$, it becomes finite and system enters into the metallic phase. Thus the critical strength of disorder for WSM-metal QPT in the bulk is $W_c = 1 \pm 0.1$, and $\varrho(0)$ can be used as bonafide OP across this transition.

Next, we focus at the QCP, located at $W = W_c$. For $W = W_c$ the scaling function for ADOS in Eq. (S6) must be independent of $\delta$, implying $F(x) \sim x^{\frac{d}{z}-1}$. Therefore, when $W = W_c$, $\varrho(E) \sim |E|^{\frac{d}{z}-1}$, and by comparing $\varrho(E)$ vs. $E$ we obtain the DSE $z$ to be $z = 1.49 \pm 0.05$ [Fig. S7B]. It is worth pointing out that numerically extracted value of the DSE from our method (highlighted in Sec. S1) matches quite well with the results obtained by using the KPM [17, 19, 21, 22, 24] and the scaling of conductance obtained via transfer matrix formalism [20].

Finally, to obtain CLE, we turn our attention to the metallic side of the transition, where ADOS at zero energy becomes finite, suggesting $F(x) \sim x^0$ (to the leading order) in the metallic phase. From the scaling function in Eq. (S6), we then obtain $\varrho(0) \sim \delta^{(d-z)\nu}$. Thus by comparing $\varrho(0)$ vs. $\delta$, we extract the CLE to be $\nu = 1.02 \pm 0.05$ [Fig. S7C]. The extracted value for the CLE matches reasonably well with the ones obtained by using KPM [17, 19, 21, 22, 24].

### B. ADOS from real space simulation using kernel polynomial method

We now present the analysis of ADOS obtained by using KPM with stacked planar construction of potential disorder or random charge impurities. Recall that in our model [Eq. (S1)], the Weyl nodes, located at $\mathbf{K}_0 = \left(0, 0, \frac{\pi}{2a}\right)$, are placed along the $\hat{z}$ direction. To test the robustness of the universality class of the WSM-metal QPT we here employ the stacked planar construction in two setups. (i) Potential disorder varies randomly and uniformly within the range $[-W, W]$ only in the $\hat{x}$ direction while it is completely uniform in the $y - z$ plane. The system size for

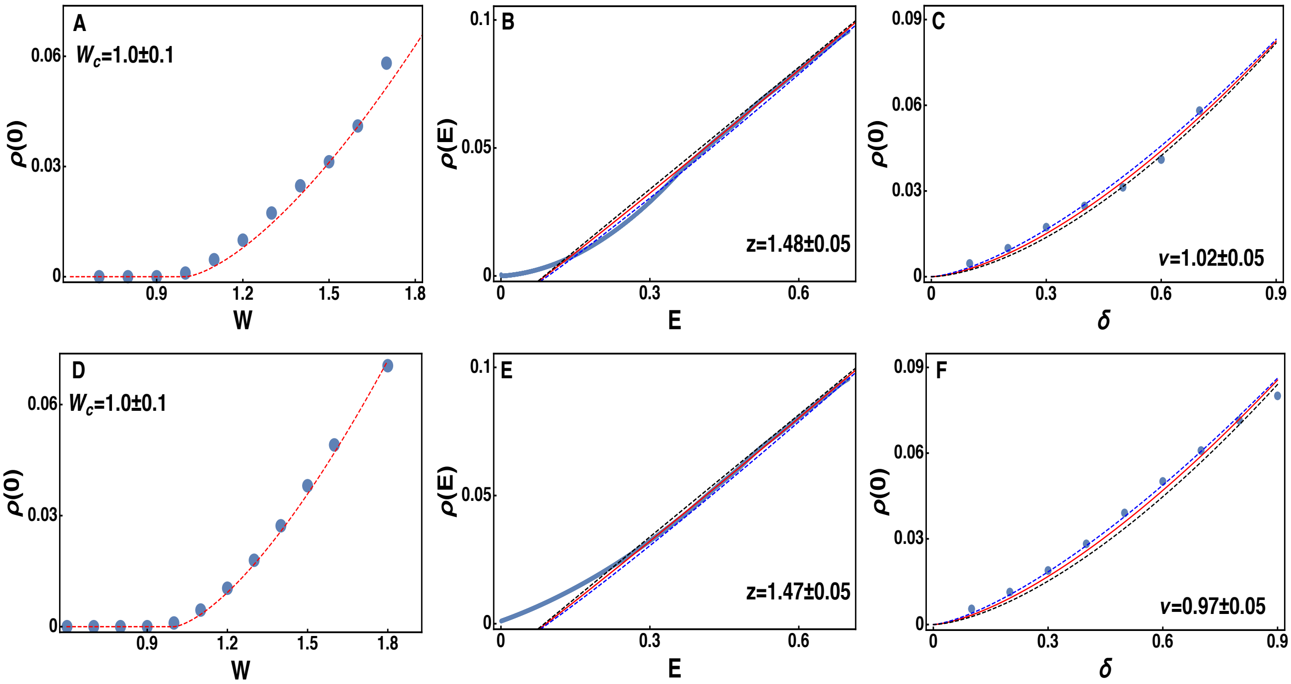


FIG. S8: Analysis of average density of states to pin the critical strength disorder ($W_c$) [panels **(A)** and **(D)**], dynamic scaling exponent ($z$) [panels **(B)** and **(E)**] and correlation length exponent ($\nu$) [panels **(C)** and **(F)**] with stacked planar construction of potential disorder that varies randomly and uniformly only in the $\hat{x}$ [panels **(A)**-**(C)**] and $\hat{z}$ [panels **(D)**-**(F)**] direction, while being constant in the orthogonal plane. The system size for the top and bottom panels is respectively $L_x \times L_y \times L_z = 3000 \times 30 \times 30$ and $L_x \times L_y \times L_z = 30 \times 30 \times 3000$.

such construction is $L_x \times L_y \times L_z = 3000 \times 30 \times 30$. (ii) Potential disorder varies randomly only in the $\hat{z}$ direction within the range $[-W, W]$. The dimension of the system for such construction is $L_x \times L_y \times L_z = 30 \times 30 \times 3000$. We perform disorder averaging over 200 independent disorder realizations. Note the system size along which disorder potential varies randomly and uniformly within the range $[-W, W]$ is 100 times larger than that in a plane where it is completely uniform. Such construction is necessary to ensure that the system is not self-doped and that net or overall chemical potential is pinned at or extremely close to the Weyl nodes. Nonetheless, we always find that ADOS for weak enough disorder scales as $\varrho(E) \sim |E|^2$ [see Fig. S6B and Fig. S6C with construction (i) and (ii), respectively], ensuring that different linear dimensionality of the system along various directions does not harm the existence of linearly dispersing Weyl fermions.

The scaling analysis of ADOS for these two constructions are respectively shown in Fig. S8 (panels A-C) and Fig. S8 (panels D-F). First note that strength of the critical disorder with either of the two constructions is $W_c = 1.0 \pm 0.1$, same (within numerical accuracy) as the one reported in the previous subsection. Following the same scaling analysis for the ADOS, discussed in the previous subsection we obtain the value of DSE and CLE with the above two disorder implementations to be (i) $z = 1.48 \pm 0.05$ [Fig. S8B], $\nu = 1.02 \pm 0.05$ [Fig. S8C], (ii) $z = 1.47 \pm 0.5$ [Fig. S8E], $\nu = 0.97 \pm 0.05$ [Fig. S8F].

Therefore, within the numerical error bar we find that any of the considered constructions for the realization of potential disorder yields same universality class of the WSM-metal QPT. We also wish to point out that when we perform the numerical analysis with KPM in a system with dimension $L_x \times L_y \times L_z = 120 \times 120 \times 120$, with disorder potential $V(\mathbf{r})$ varying randomly and uniformly within the range $[-W, W]$ in all three directions, we find $W_c = 1.75 \pm 0.1$ [Fig. S9A], $z = 1.49 \pm 0.05$ [Fig. S9B] and $\nu = 0.98 \pm 0.05$ [Fig. S9C]. Therefore, different distributions of the disorder potential only cause a nonuniversal shift of the location of the WSM-metal QCP, without changing its universality class. These observations, together with the result we discuss in the next section provide extremely strong support in favor of the bulk-boundary correspondence across the WSM-metal QPT.

As a final remark, we point out that in our numerical analysis there is always a finite but small offset of ADOS near zero energy even for a subcritical strength of disorder, which is, however, a common feature of this analysis that has

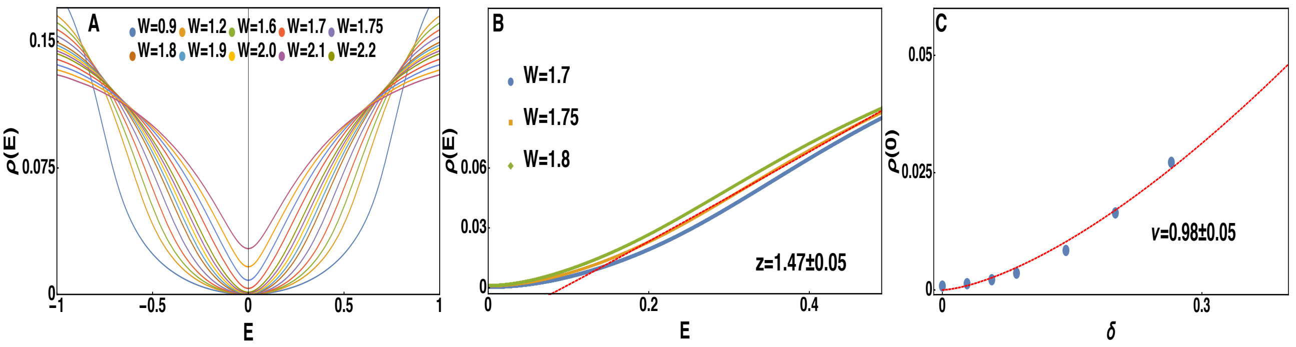


FIG. S9: **(A)** Scaling of average density of states in an increasingly disordered Weyl semimetal, where disorder potential $V(\mathbf{r})$ varies randomly and uniformly within $[-W, W]$ at each site of the cubic lattice. Critical strength of disorder for Weyl semimetal-metal quantum phase transition is $W_c = 1.75 \pm 0.05$. **(B)** Extraction of dynamic scaling exponent $(z)$, yielding $z = 1.47 \pm 0.05$. **(C)** Extraction of correlation length exponent $(\nu)$, yielding $\nu = 0.98 \pm 0.05$.

also been reported in Refs. [17, 19, 21, 22, 24]. Nevertheless, such offset gradually decreases with increasing system size (along which the disorder varies randomly in the stacked planar construction) and number of disorder averaging. For data analysis we subtract such finite but small offset, and reconstruct the ADOS by following its scaling within the range $0.05t \leq |E| \leq 0.4t$, as the signature of disorder-driven quantum critical regime is most pronounced and reliable in this interval of energies. However, even without such subtraction, we observe a clear $\varrho(E) \sim |E|^2$ scaling for $W \ll 1$ and $\varrho(E) \sim |E|$ around $W = 1.0$ at finite energies ($|E| > 0.05\,t$). These results guarantee the robustness of a sharp WSM-metal QCP around $W = W_c = 1.0 \pm 0.1$. Now we proceed with a quantitative analysis of the dissolution of the topological Fermi arc with increasing disorder in the WSM.

## S3. FERMI ARC STATES FOR THE SYSTEMS OF THE LINEAR SIZE $L = 100$ AND $L = 200$ IN THE OPEN DIRECTION

In this Section, we focus on systems with linear dimension $L = 100$ (Fig. S2, Fig. S4) and $L = 200$ (Fig. S3, Fig. S5) in the $\hat{x}$ direction, along which we impose open boundary, and present evolution of one-dimensional chiral edge states on the top surface (Fig. S2 and Fig. S3) and variation of the fraction of the wavefunction for the same set of the surface states (Fig. S4 and Fig. S5) with increasing disorder. Recall that the Fermi arc can be constructed by joining the locus of the zero energy mode of the chiral edge states. The results are qualitatively the same as for the system size $L = 300$, presented in the main text. Most importantly, the Fermi arcs dissolve into the metallic bath in the bulk at the disorder strength $W = W_* < W_c$, with $W_* \simeq 0.8 - 0.9$, in the same range as that for the system size $L = 300$. This observation is consistent with the scaling arguments presented in the main text, which we elaborate here. In addition, from the scaling analysis we can roughly estimate the strength of disorder $W_*$ for which the Fermi arc dissolves into the bulk metallic bath, as discussed below. Estimated values for $W_*$ in various systems with linear dimension $L$ along the open boundary direction match reasonably well the numerically estimated value of $W_*$.

We can roughly estimate the strength of disorder $(W_*)$ at which Fermi arc state looses its support on the surface in the following way. It should be noted that $W_*$ defines only a crossover boundary between the semimetallic to quantum critical regime in a finite size system. Recall that we expect the dissolution of the arcs to take place when the correlation length

$$\xi \sim \left(\frac{W_c - W_*}{W_c}\right)^{-\nu} \sim L, \tag{S7}$$

which allows us to estimate $W_*$ as linear dimension $L$ varies. Both $\xi$ and $L$ are conveniently measured in units of the lattice spacing $a$. Now we can set $W_c = 1$ [Fig. S7A], and for the sake of simplicity we assume $\nu = 1$, consistent with numerically extracted value [Fig. S7C]. It should be noted that there is a dimensionless non-universal constant $(c)$ that enters in the definition of the correlation length according to $\xi = c\left(\frac{W_c - W}{W_c}\right)^{-\nu}$, which can be estimated (roughly) in

the following way. From the data presented in Fig. 2 and Fig. 3 of the main text, we estimate $W_* = 0.9$ for $L = 300$, yielding $c = 30$. From the estimated value of the non-universal constant $c = 30$, we then obtain $W_* = 0.85$ for $L = 200$ and $W_* = 0.7$ for $L = 100$. From Figs. S2, S3, S4, S5, we find that the Fermi arc dissolves into the metallic bath for $W_* = 0.8(\pm 0.1)$ in systems with linear dimension $L = 100$ and 200 (along which we implement open boundary), which within our numerical error bar agrees with the estimation for $W_*$.

---


[1] E. Fradkin, *Critical behavior of disordered degenerate semiconductors. II. Spectrum and transport properties in mean-field theory*, Phys. Rev. B **33**, 3263 (1985).

[2] R. Shindou, and S. Murakami, *Effects of disorder in three-dimensional $Z_2$ quantum spin Hall systems*, Phys. Rev. B **79**, 045321 (2009).

[3] P. Goswami, and S. Chakravarty, *Quantum Criticality between Topological and Band Insulators in $3+1$ Dimensions*, Phys. Rev. Lett. **107**, 196803 (2011).

[4] Y. Ominato, and M. Koshino, *Quantum transport in a three-dimensional Weyl electron system*, Phys. Rev. B **89**, 054202 (2014).

[5] B. Roy, and S. Das Sarma, *Diffusive Quantum Criticality in Three Dimensional Disordered Dirac Semimetals*, Phys. Rev. B **90**, 241112(R) (2014).

[6] S. V. Syzranov, L. Radzihovsky, V. Gurarie, *Critical Transport in Weakly Disordered Semiconductors and Semimetals*, Phys. Rev. Lett. **114**, 166601 (2015).

[7] A. Altland, and D. Bagrets, *Effective Field Theory of the Disordered Weyl Semimetal*, Phys. Rev. Lett. **114**, 257201 (2015).

[8] B. Roy, S. Das Sarma, *Quantum phases of interacting electrons in three-dimensional dirty Dirac semimetals*, Phys. Rev. B **94**, 115137 (2016).

[9] B. Roy, V. Juričić, S. Das Sarma, *Universal optical conductivity of a disordered Weyl semimetal*, Sci. Rep. **6**, 32446 (2016).

[10] T. Louvet, D. Carpentier, A. A. Fedorenko, *On the disorder-driven quantum transition in three-dimensional relativistic metals*, Phys. Rev. B **94**, 220201 (2016).

[11] S. V. Syzranov, V. Gurarie, L. Radzihovsky, *Multifractality at non-Anderson disorder-driven transitions in Weyl semimetals and other systems*, Ann. Phys. **373**, 694 (2016)

[12] A. K. Mitchell, and L. Fritz, *Signatures of Weyl semimetals in quasiparticle interference*, Phys. Rev. B **93**, 035137 (2016).

[13] E. V. Gorbar, V. A. Miransky, I. A. Shovkovy, and P. O. Sukhachov, *Origin of dissipative Fermi arc transport in Weyl semimetals*, Phys. Rev. B **93**, 235127 (2016).

[14] T. Louvet, D. Carpentier, A. A. Fedorenko, *New Quantum Transition in Weyl Semimetals with Correlated Disorder*, Phys. Rev. B **95**, 014204 (2017).

[15] B. Roy, R-J. Slager, V. Juričić, *Global phase diagram of a dirty Weyl semimetal*, arXiv:1610.08973

[16] P. Goswami, S. Chakravarty, *Superuniversality of topological quantum phase transition and global phase diagram of dirty topological systems in three dimensions*, Phys. Rev. B **95**, 075131 (2017).

[17] K. Kobayashi, T. Ohtsuki, K-I. Imura, I. F. Herbut, *Density of States Scaling at the Semimetal to Metal Transition in Three Dimensional Topological Insulators*, Phys. Rev. Lett. **112**, 016402 (2014).

[18] B. Sbierski, G. Pohl, E. J. Bergholtz, P. W. Brouwer, *Quantum Transport of Disordered Weyl Semimetals at the Nodal Point*, Phys. Rev. Lett. **113**, 026602 (2014).

[19] J. H. Pixley, P. Goswami, and S. Das Sarma, *Anderson Localization and the Quantum Phase Diagram of Three Dimensional Disordered Dirac Semimetals*, Phys. Rev. Lett. **115**, 076601 (2015).

[20] B. Sbierski, E. J. Bergholtz, P. W. Brouwer, *Quantum critical exponents for a disordered three-dimensional Weyl node*, Phys. Rev. B **92**, 115145 (2015).

[21] J. H. Pixley, P. Goswami, and S. Das Sarma, *Disorder-driven itinerant quantum criticality of three-dimensional massless Dirac fermions*, Phys. Rev. B **93**, 085103 (2016).

[22] S. Liu, T. Ohtsuki, R. Shindou, *Effect of Disorder in a Three-Dimensional Layered Chern Insulator*, Phys. Rev. Lett. **116**, 066401 (2016).

[23] C-Z. Chen, J. Song, H. Jiang, Q-F Sun, Z. Wang, X. C. Xie, *Disorder and Metal-Insulator Transitions in Weyl Semimetals*, Phys. Rev. Lett. **115**, 246603 (2015).

[24] S. Bera, J. D. Sau, and B. Roy, *Dirty Weyl semimetals: Stability, phase transition, and quantum criticality*, Phys. Rev. B **93**, 201302 (2016).

[25] H. Shapourian, T. L. Hughes, *Phase diagrams of disordered Weyl semimetals*, Phys. Rev. B **93**, 075108 (2016).

[26] B. Roy, Y. Alavirad, J. D. Sau, *Global phase diagram of a three dimensional dirty topological superconductor*, arXiv:1604.01390

[27] Z. Huang, T. Das, A. V. Balatsky, and D. P. Arovas, *Stability of Weyl metals under impurity scattering*, Phys. Rev. B **87**, 155123 (2013).

[28] R. Nandkishore, D. A. Huse, S. L. Sondhi, *Rare region effects dominate weakly disordered three-dimensional Dirac points*, Phys. Rev. B **89**, 245110 (2014).

[29] J. H. Pixley, D. A. Huse, S. Das Sarma, *Rare-Region-Induced Avoided Quantum Criticality in Disordered Three-Dimensional Dirac and Weyl Semimetals*, Phys. Rev. X **6**, 021042 (2016).

[30] J. H. Pixley, Y-Z. Chou, P. Goswami, D. A. Huse, R. Nandkishore, L. Radzihovsky, S. Das Sarma, *Single particle excitations*

*in disordered Weyl fluids*, arXiv:1701.00783

[31] B. Fu, W. Zhu, Q. Shi, Q. Li, J. Yang, and Z. Zhang, *Accurate Determination of the Quasiparticle and Scaling Properties Surrounding the Quantum Critical Point of Disordered Three-Dimensional Dirac Semimetals*, Phys. Rev. Lett. **118**, 146401 (2017).

[32] A. Weiße, G. Wellein, A. Alvermann, and H. Fehske, *The kernel polynomial method*, Rev. Mod. Phys. **78**, 275 (2006).
